# Supplementary material for: DA-Code: Agent Data Science Code Generation Benchmark for Large Language Models
Source: arXiv:2410.07331 source file (2024-10-11)
Supplement: Supplementary file 1 [file image_information.tex]

%\section{Image Information Description}
%\label{app:image information}

%In this section, we will introduce the image information involved in data visualization tasks in %\ours using an example that includes all the relevant information:

%\begin{figure}[htbp]
%    \centering
%    \includegraphics[width=0.9\textwidth]{figs/image_information.png}
%    \caption{Example in data visualization task}
%    \label{fig:visualization_example}
%\end{figure}

%\paragraph{figsize}Specifies the shape or dimensions of the image. It determines the width and %height of the plot in inches. In our example, it is set to (10, 6) (not explicitly shown in the image, but set in the code).
%\paragraph{color}Represents the color scheme used within the graph or visualization. It defines the hues applied to different data elements for differentiation or emphasis, like blue and orange in the example above.
%\paragraph{graph\_title}Provides the overarching title or caption for the graph. It succinctly summarizes the purpose or main findings depicted in the visual representation, for example, ``Comparison of Animal Counts in the group''.
%\paragraph{legend\_title}Describes the title of the legend, which typically explains the meaning of different colors or symbols used in the graph. It aids in understanding the data categories or groups represented, such as ``Animal''.
%\paragraph{labels}Refers to the labels associated with the visualized data points or categories. These labels provide context for interpreting the data. In the example above, it is ``Cat'' and ``Dog''.
%\paragraph{x\_label}Indicates the title for the x-axis, representing the horizontal dimension of the graph. It clarifies what the x-axis measures or represents, e.g., ``Group''.
%\paragraph{y\_label}Represents the title for the y-axis, which denotes the vertical dimension of the graph. It clarifies what the y-axis measures or represents, e.g., ``Count''.
%\paragraph{xtick\_labels} Refers to the specific labels assigned to individual ticks or points along the x-axis. These labels provide scale and context to the data points plotted on the x-axis, e.g., ``Group 1'', ``Group 2'', ``Group 3'', ``Group 4'', ``Group 5''.
%\paragraph{ytick\_labels}Represents the specific labels assigned to ticks or points along the y-axis. Similar to xtick\_labels, these labels provide scale and context to the data points plotted on the y-axis, e.g., 0, 5, 10, 15, 20, 25, 30, 35.
